# Supplementary material for: RCA-NOC: Relative Contrastive Alignment for Novel Object Captioning
Source: arXiv:2312.06299 source file (2023-12-11)
Supplement: Supplementary file 1 [file framework.pdf]

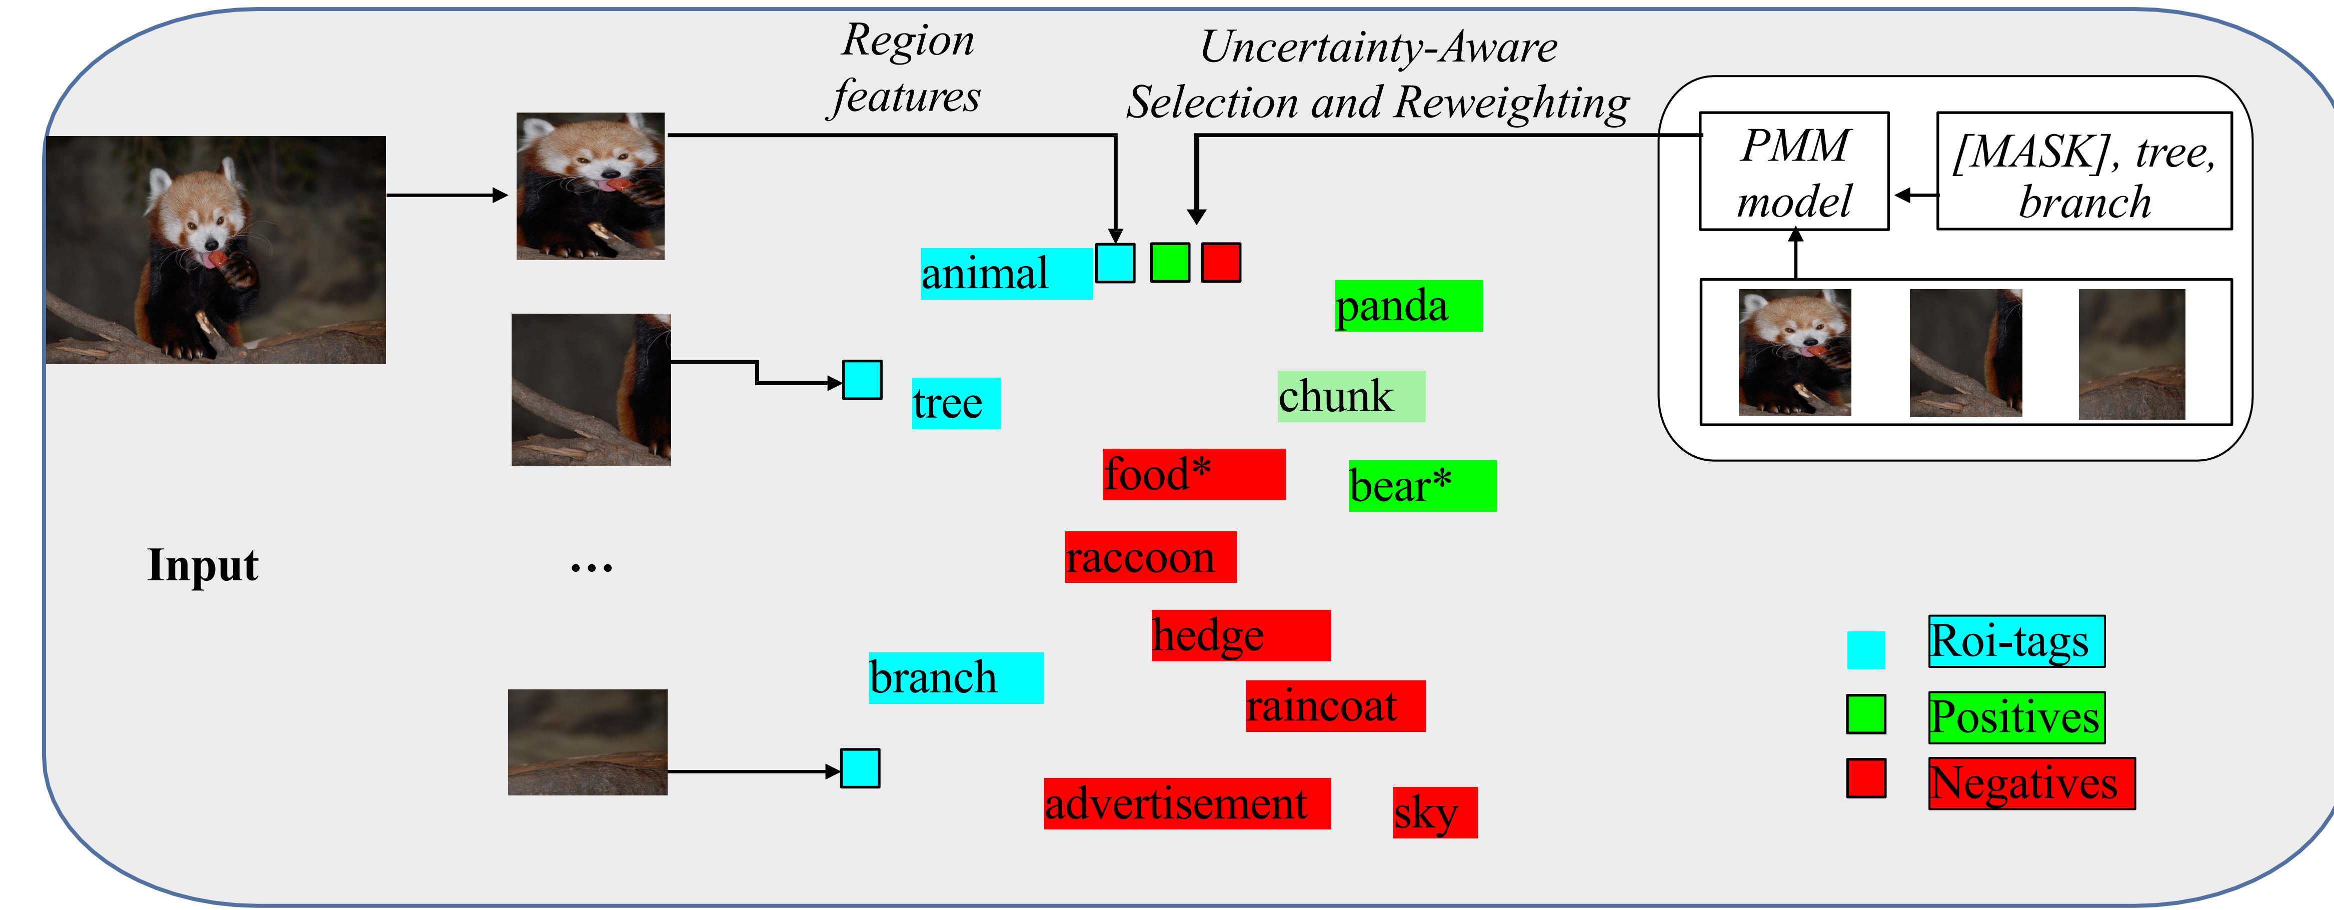
Region features
Uncertainty-Aware Selection and Reweighting
PMM model
[MASK], tree, branch
animal
panda
tree
chunk
food*
bear*
Input
...
raccoon
hedge
branch
raincoat
advertisement
sky
Roi-tags
Positives
Negatives

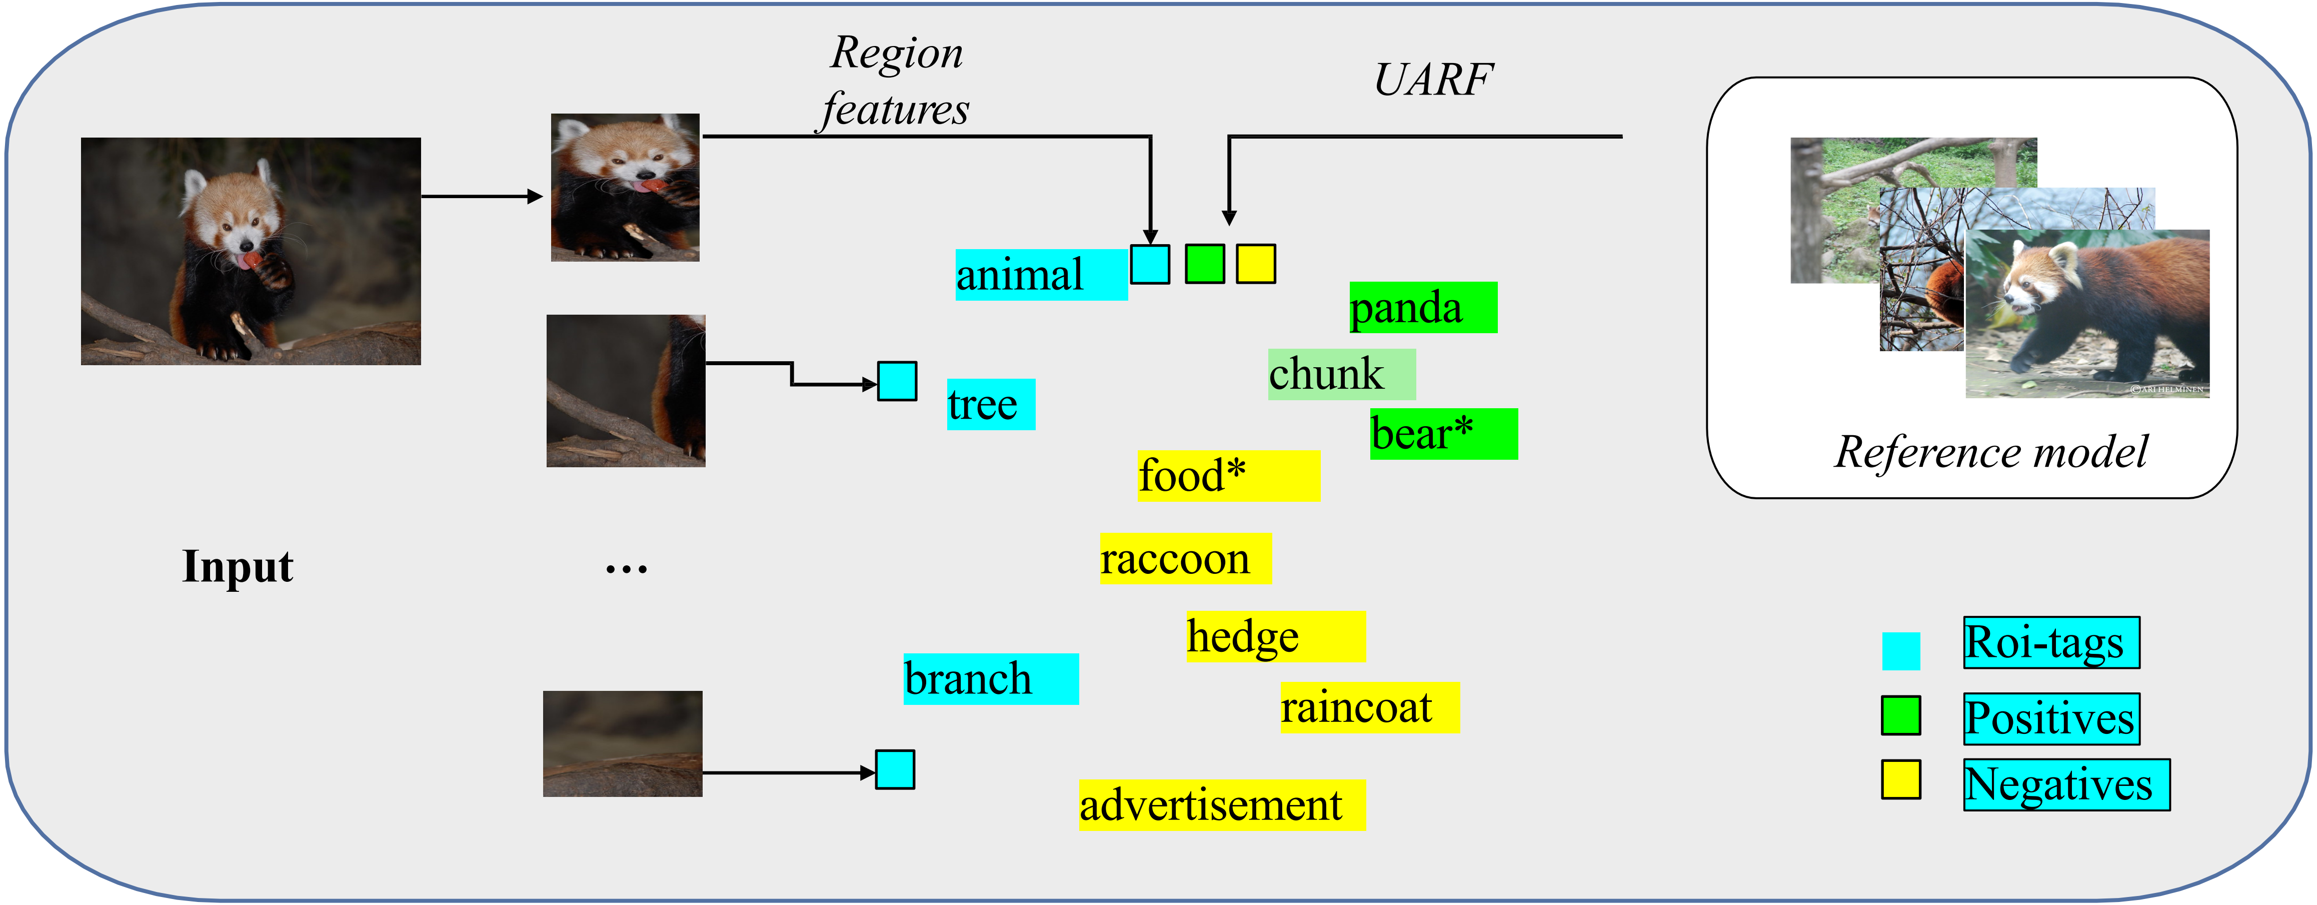
Region
features
UARF
Input
...
animal
tree
branch
panda
chunk
bear*
food*
raccoon
hedge
raincoat
advertisement
Reference model
Roi-tags
Positives
Negatives

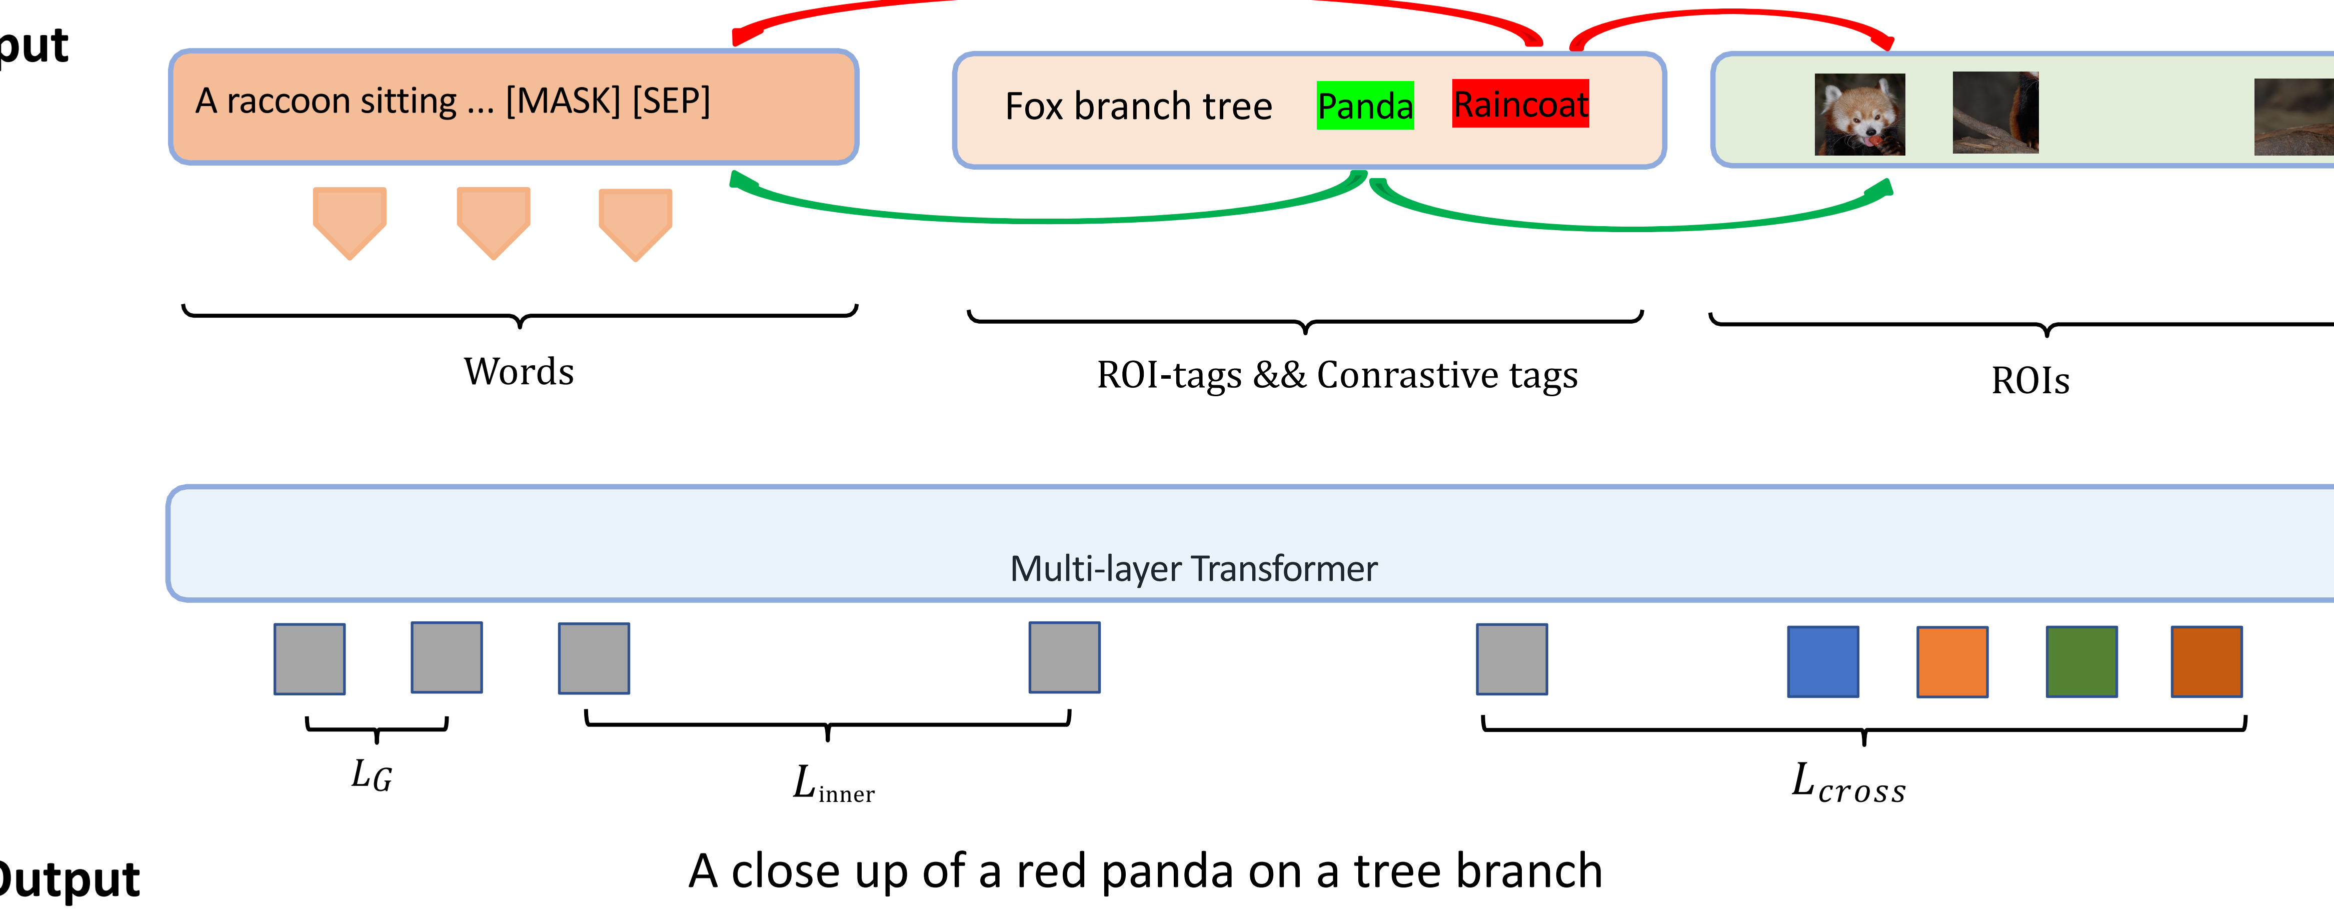

put
A raccoon sitting ... [MASK] [SEP]
Fox branch tree
Panda
Raincoat
Words
ROI-tags && Conrastive tags
ROIs
Multi-layer Transformer
$L_G$
$L_{\text{inner}}$
$L_{cross}$
utput
A close up of a red panda on a tree branch

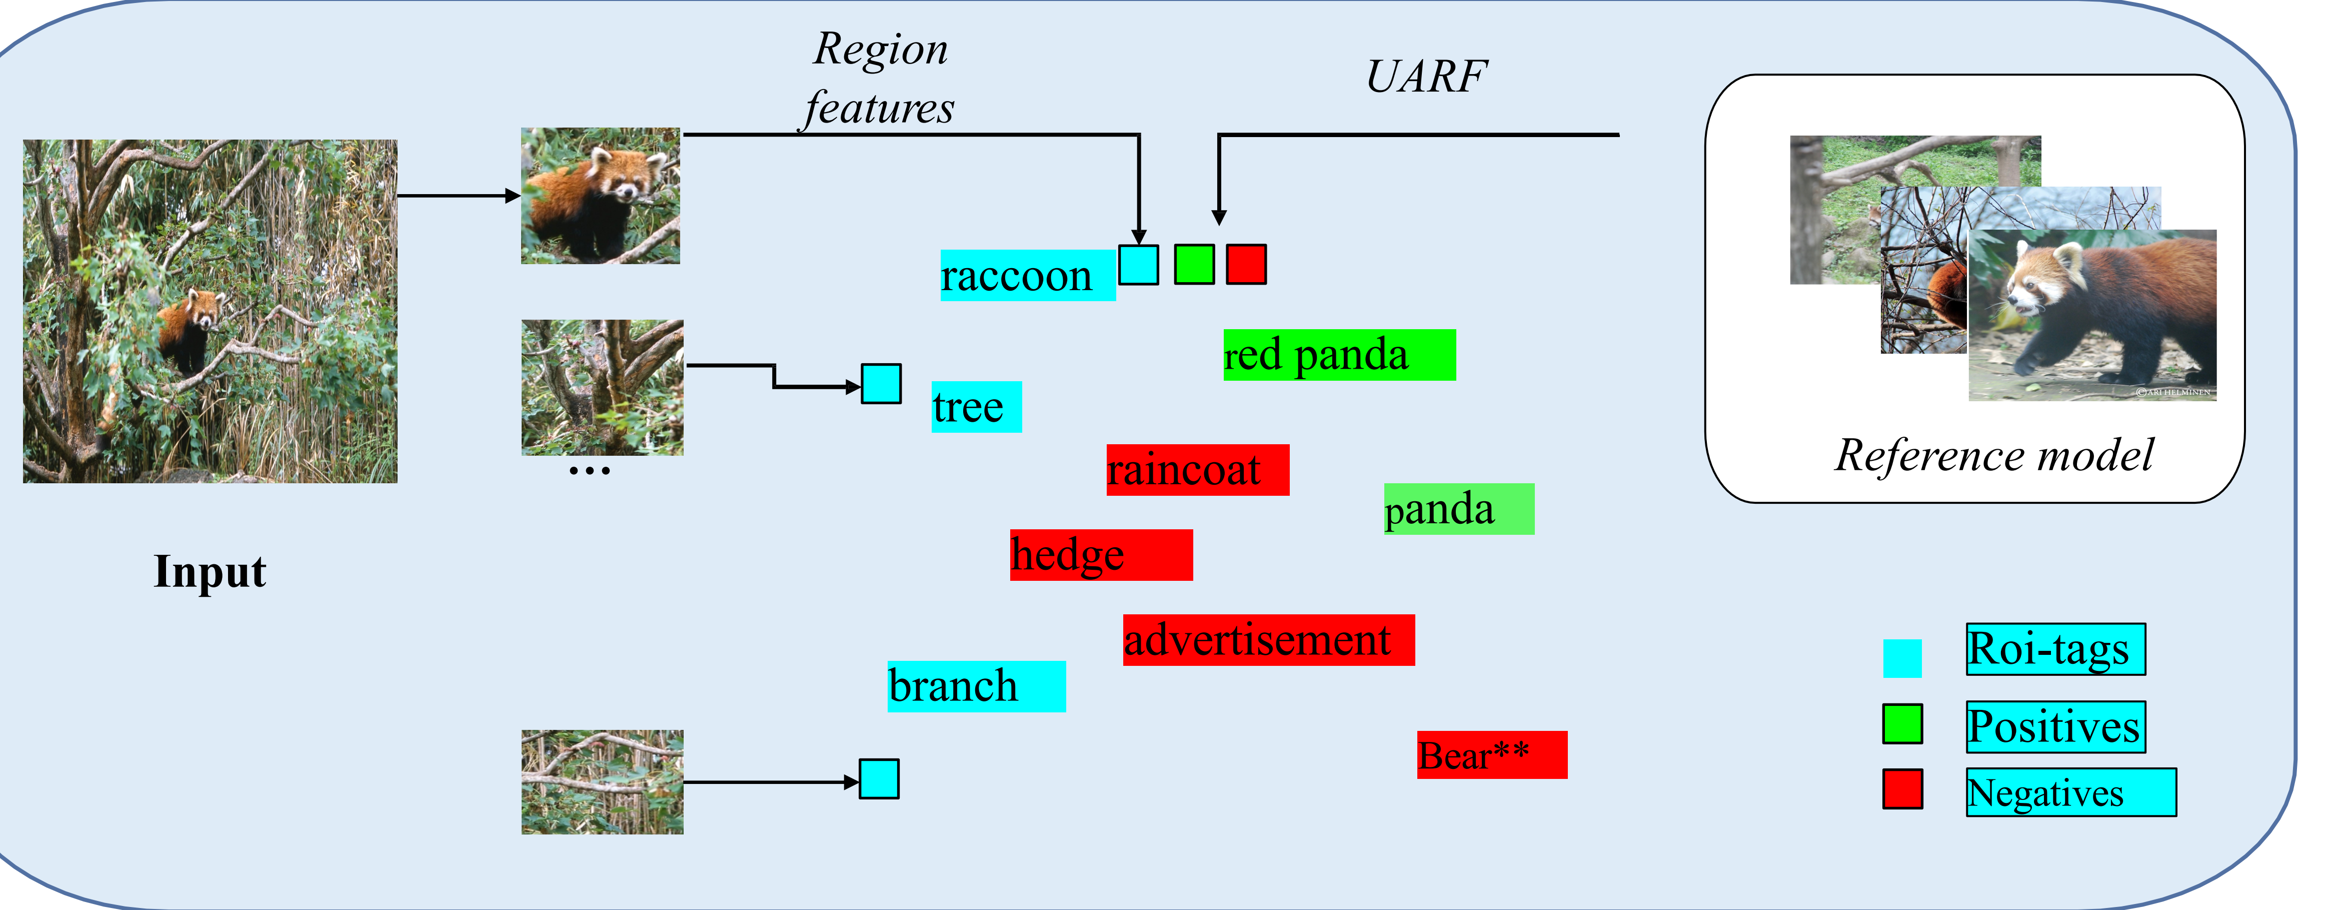

Region features
UARF
Reference model
raccoon
red panda
tree
raccoon
raincoat
panda
hedge
advertisement
branch
Bear**
Input
Roi-tags
Positives
Negatives

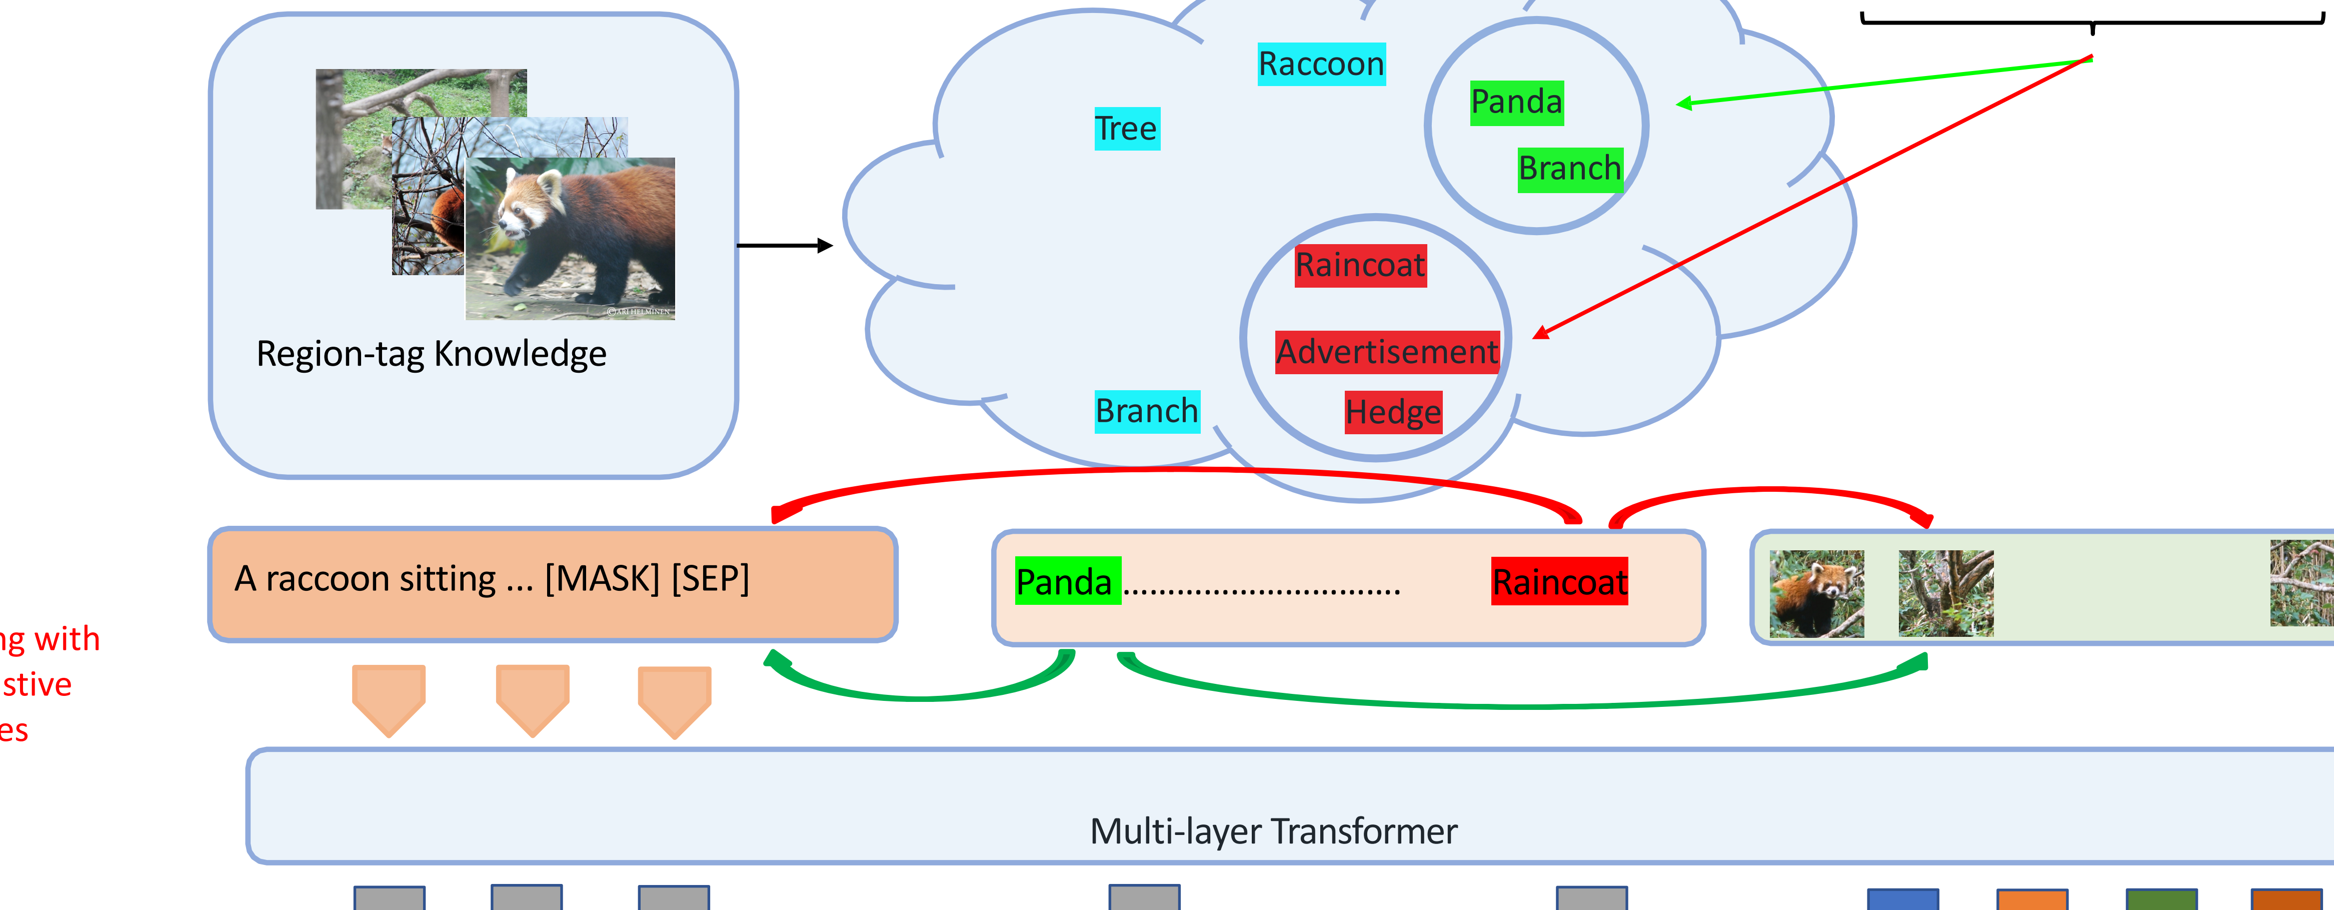
Region-tag Knowledge
Raccoon
Tree
Panda
Branch
Raincoat
Advertisement
Branch
Hedge
A raccoon sitting ... [MASK] [SEP]
Panda ..............................
Raincoat
ng with
stive
es
Multi-layer Transformer

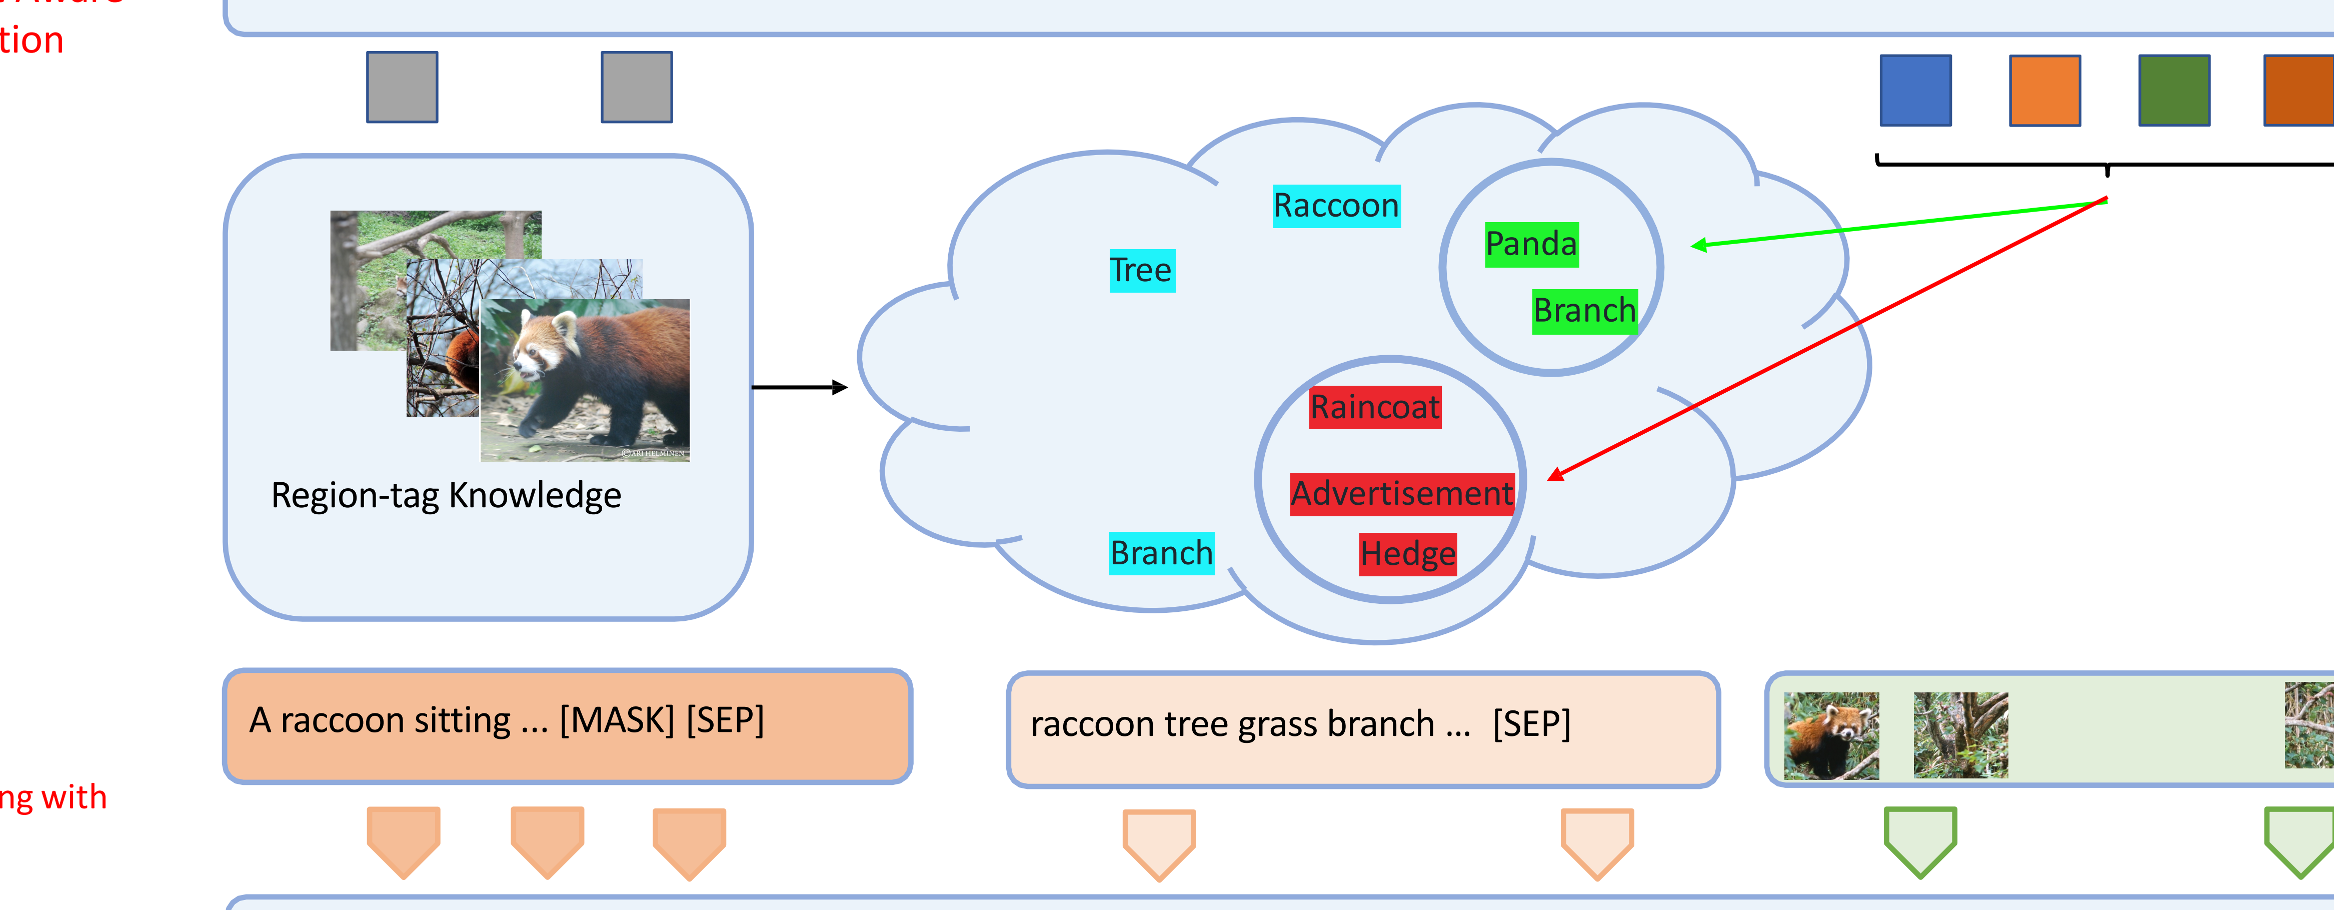

tion
Region-tag Knowledge
Raccoon
Tree
Panda
Branch
Raincoat
Advertisement
Branch
Hedge
A raccoon sitting ... [MASK] [SEP]
raccoon tree grass branch ... [SEP]
ng with

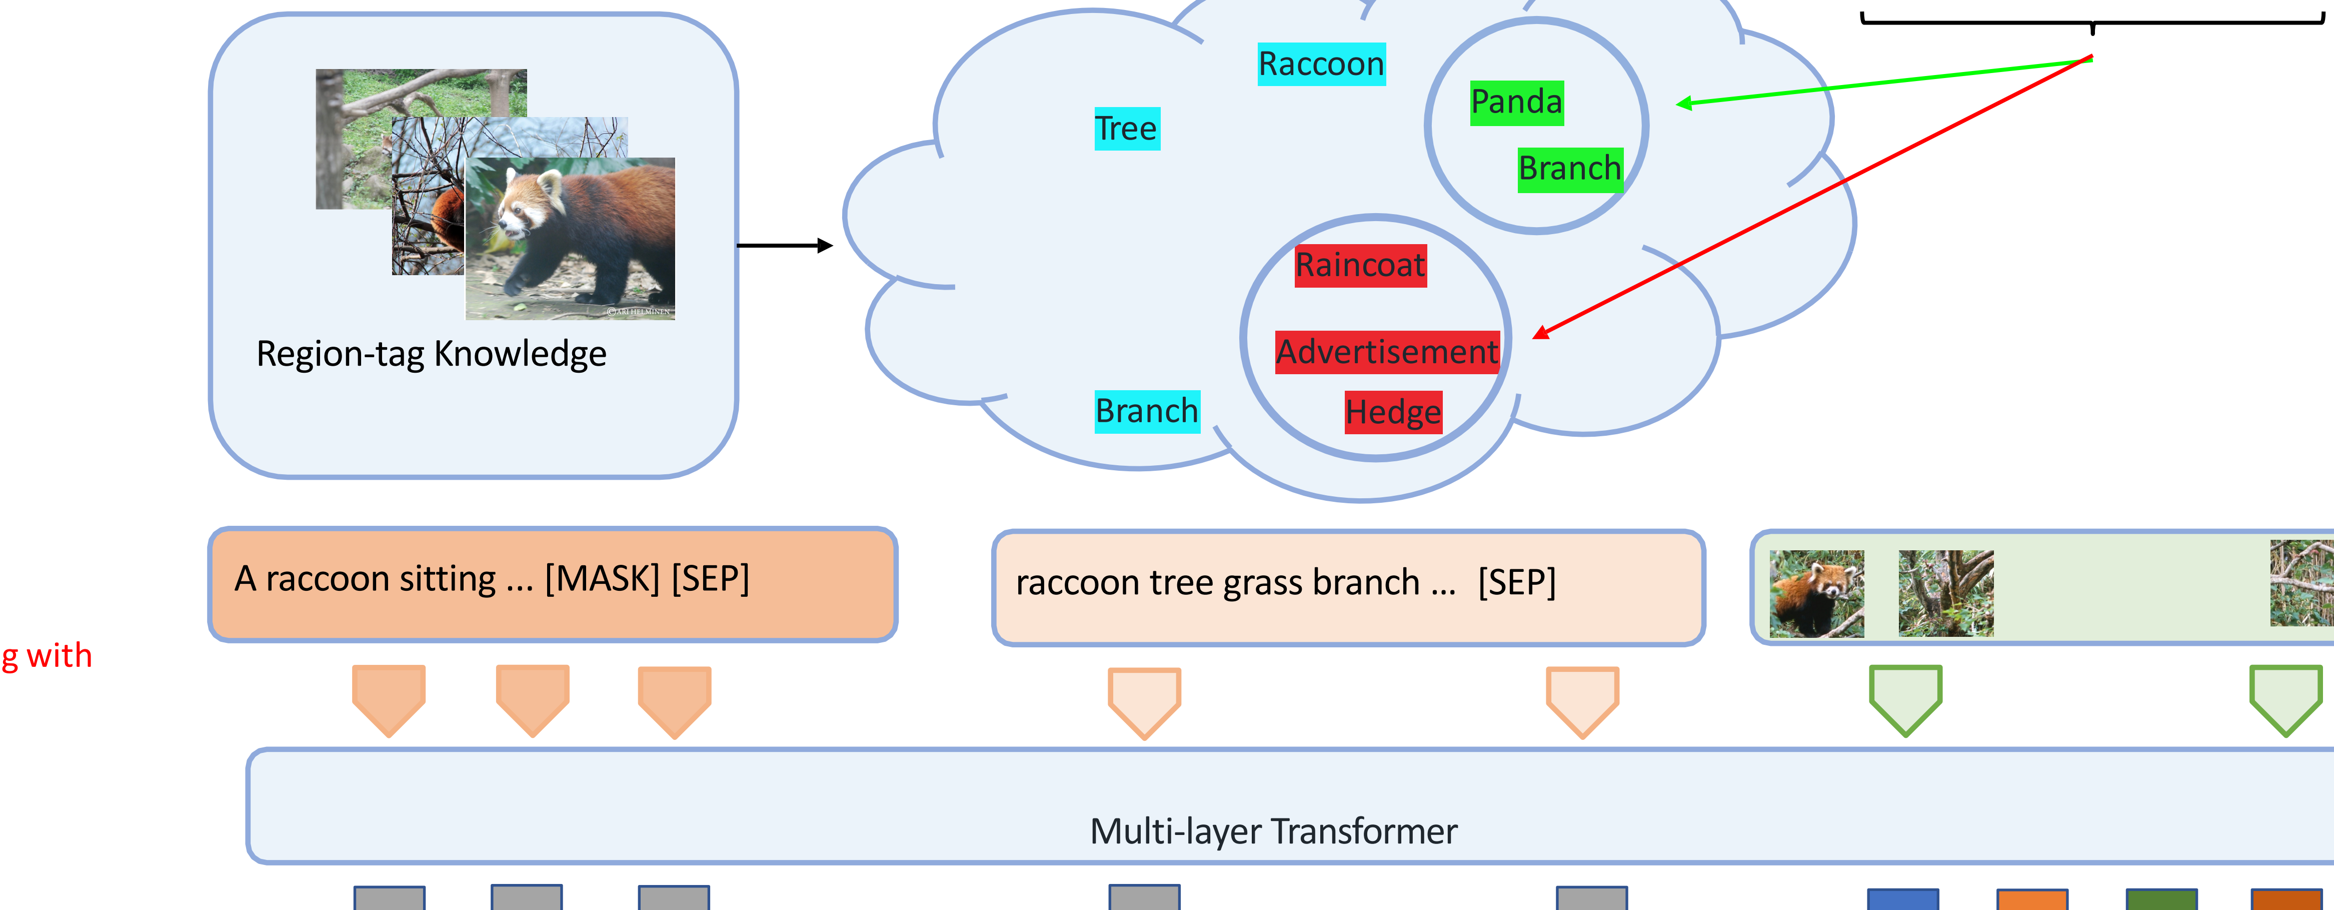
Raccoon
Tree
Panda
Branch
Raincoat
Advertisement
Branch
Hedge
Region-tag Knowledge
A raccoon sitting ... [MASK] [SEP]
raccoon tree grass branch ... [SEP]
g with
Multi-layer Transformer

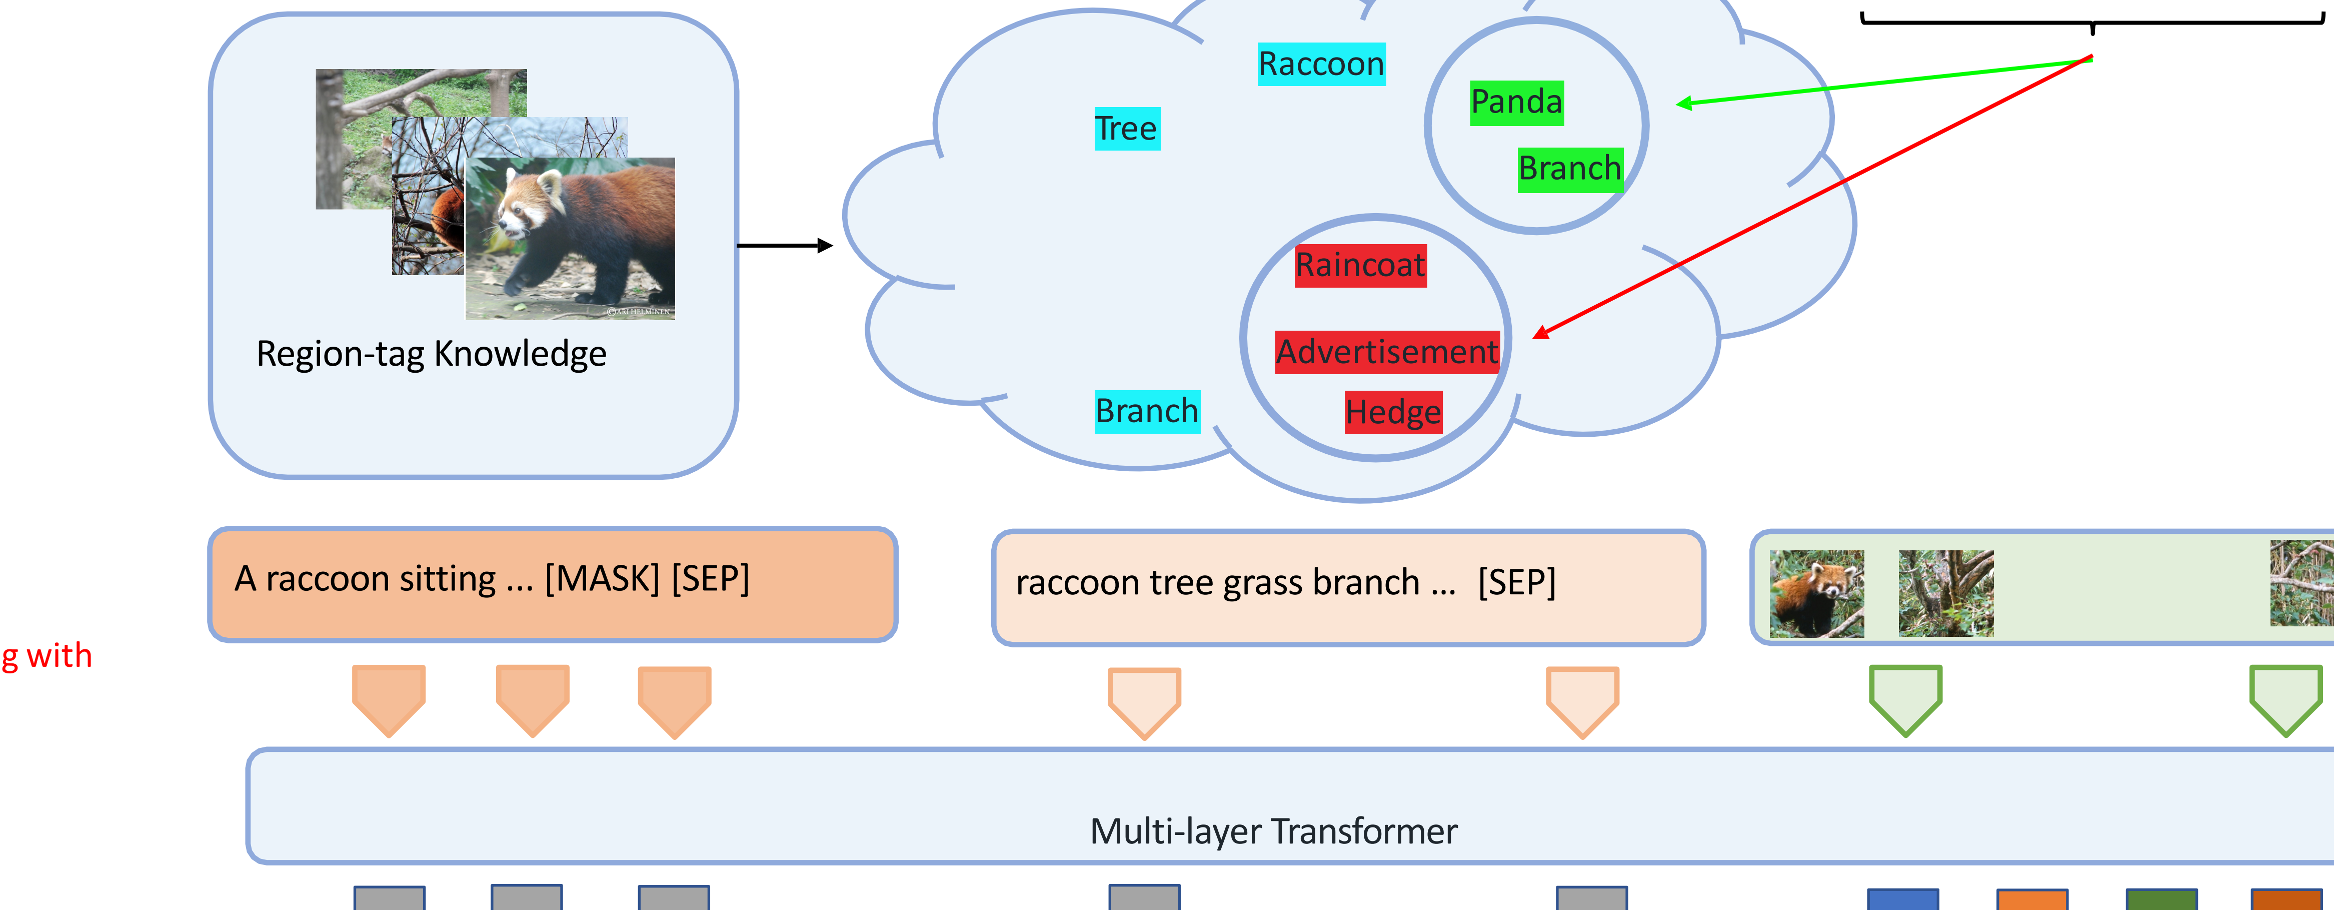
Region-tag Knowledge
Raccoon
Tree
Panda
Branch
Raincoat
Advertisement
Branch
Hedge
A raccoon sitting ... [MASK] [SEP]
raccoon tree grass branch ... [SEP]
g with
Multi-layer Transformer

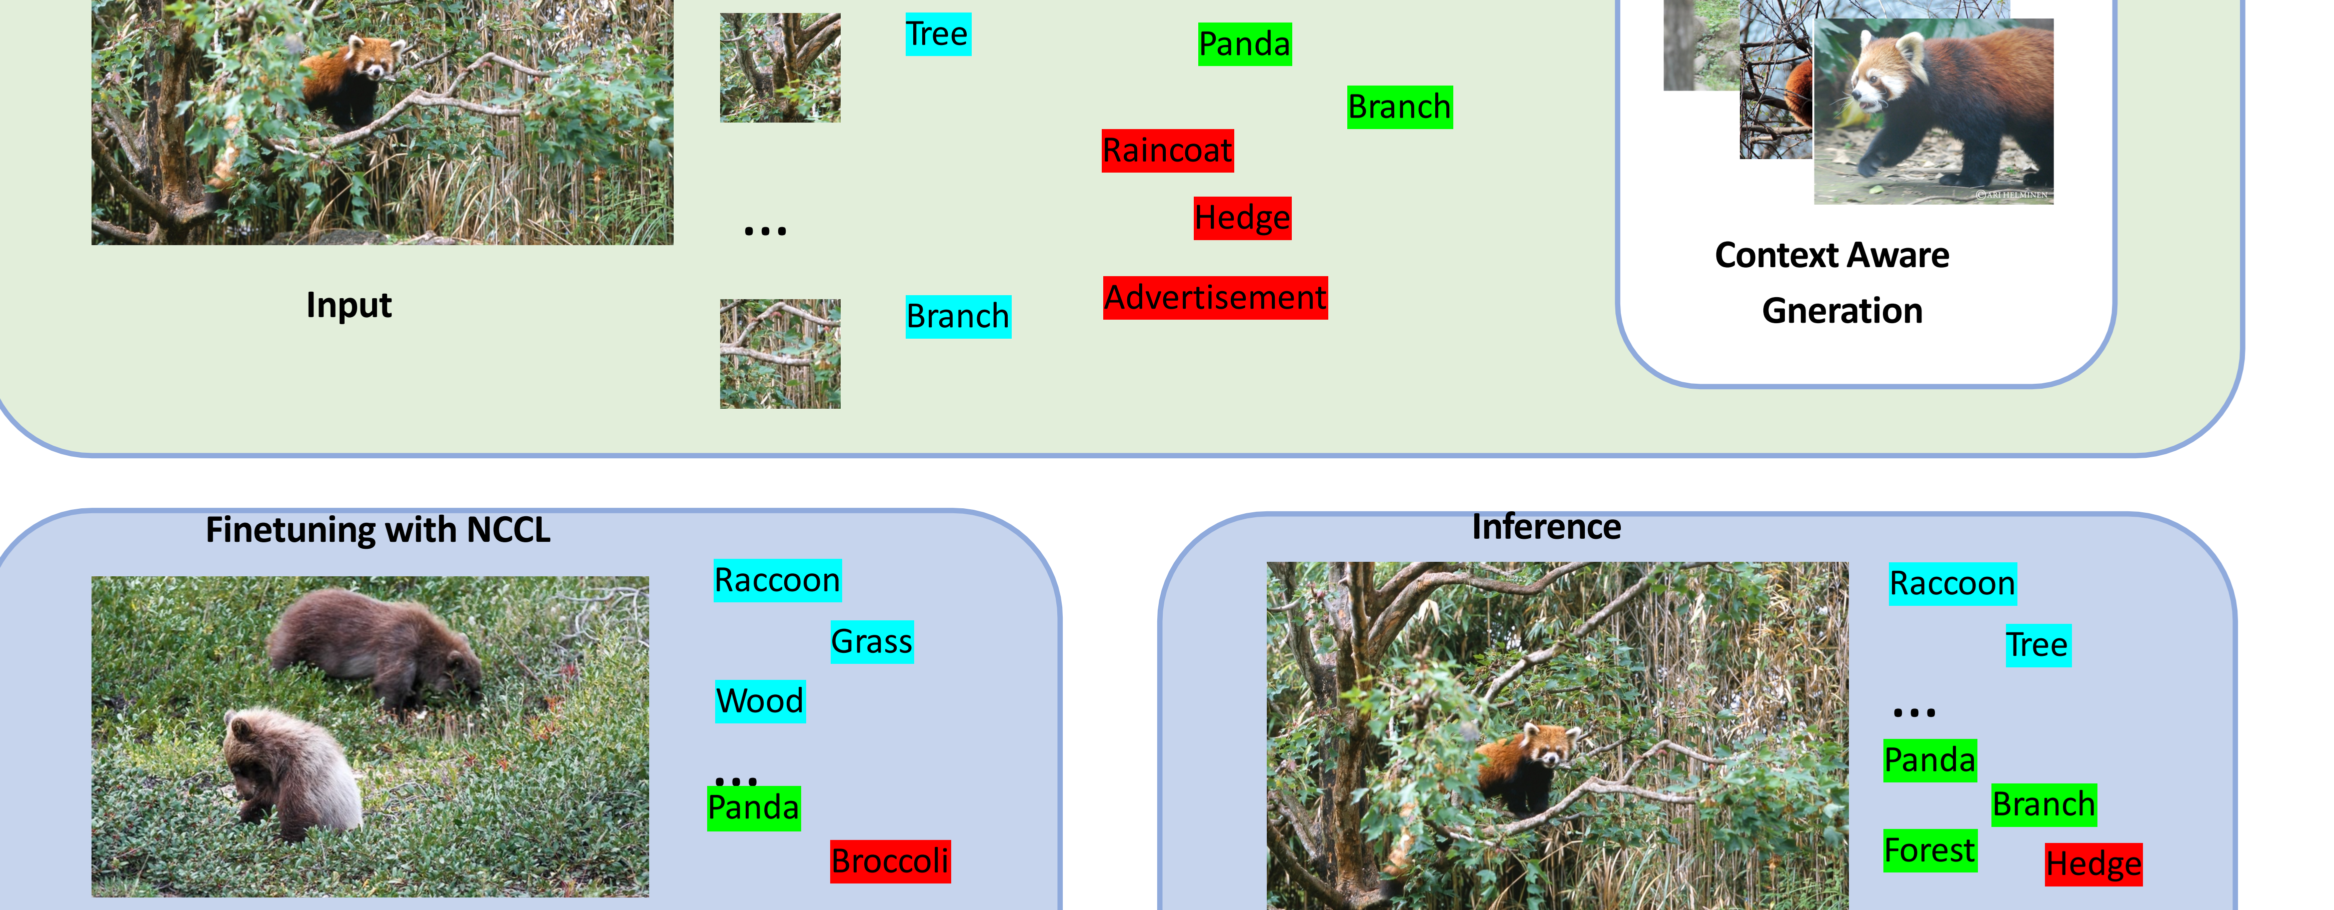

Input
Tree
Branch
Panda
Branch
Raincoat
Hedge
Advertisement
Context Aware
Gneration
Finetuning with NCCL
Raccoon
Grass
Wood
Panda
Broccoli
Inference
Raccoon
Tree
Panda
Branch
Forest
Hedge

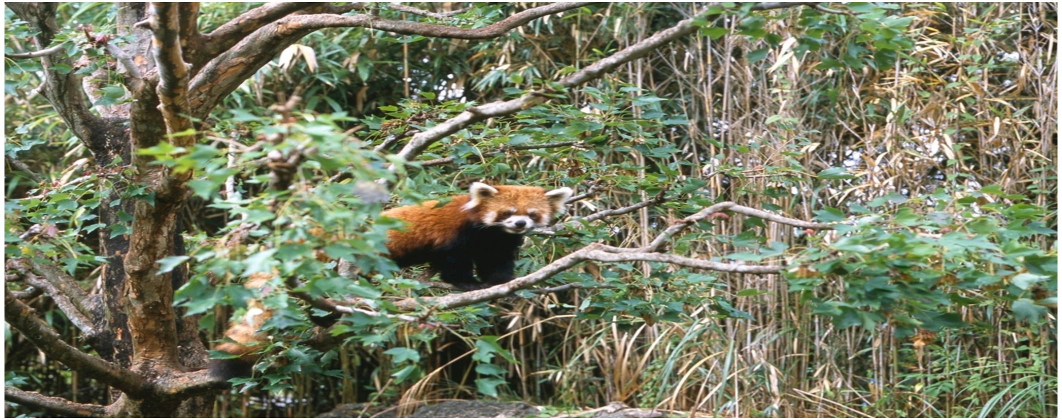

rence: Red panda sitting on the branch of a tree

/L+VIVO: A raccoon sitting in a tree.

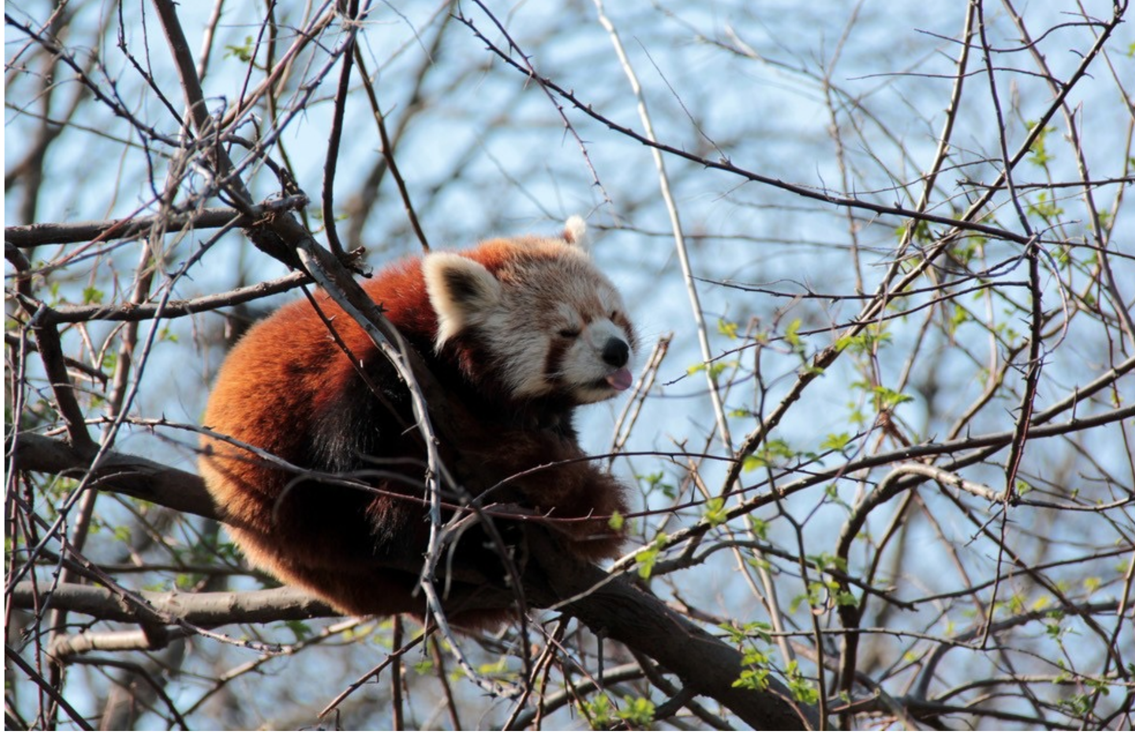

Reference: A red panda sits on a tree branch with its eyes cl

VINVL+VIVO: a raccoon sitting in a tree with no leave
