# Supplementary material for: RCA-NOC: Relative Contrastive Alignment for Novel Object Captioning
Source: arXiv:2312.06299 source file (2023-12-11)

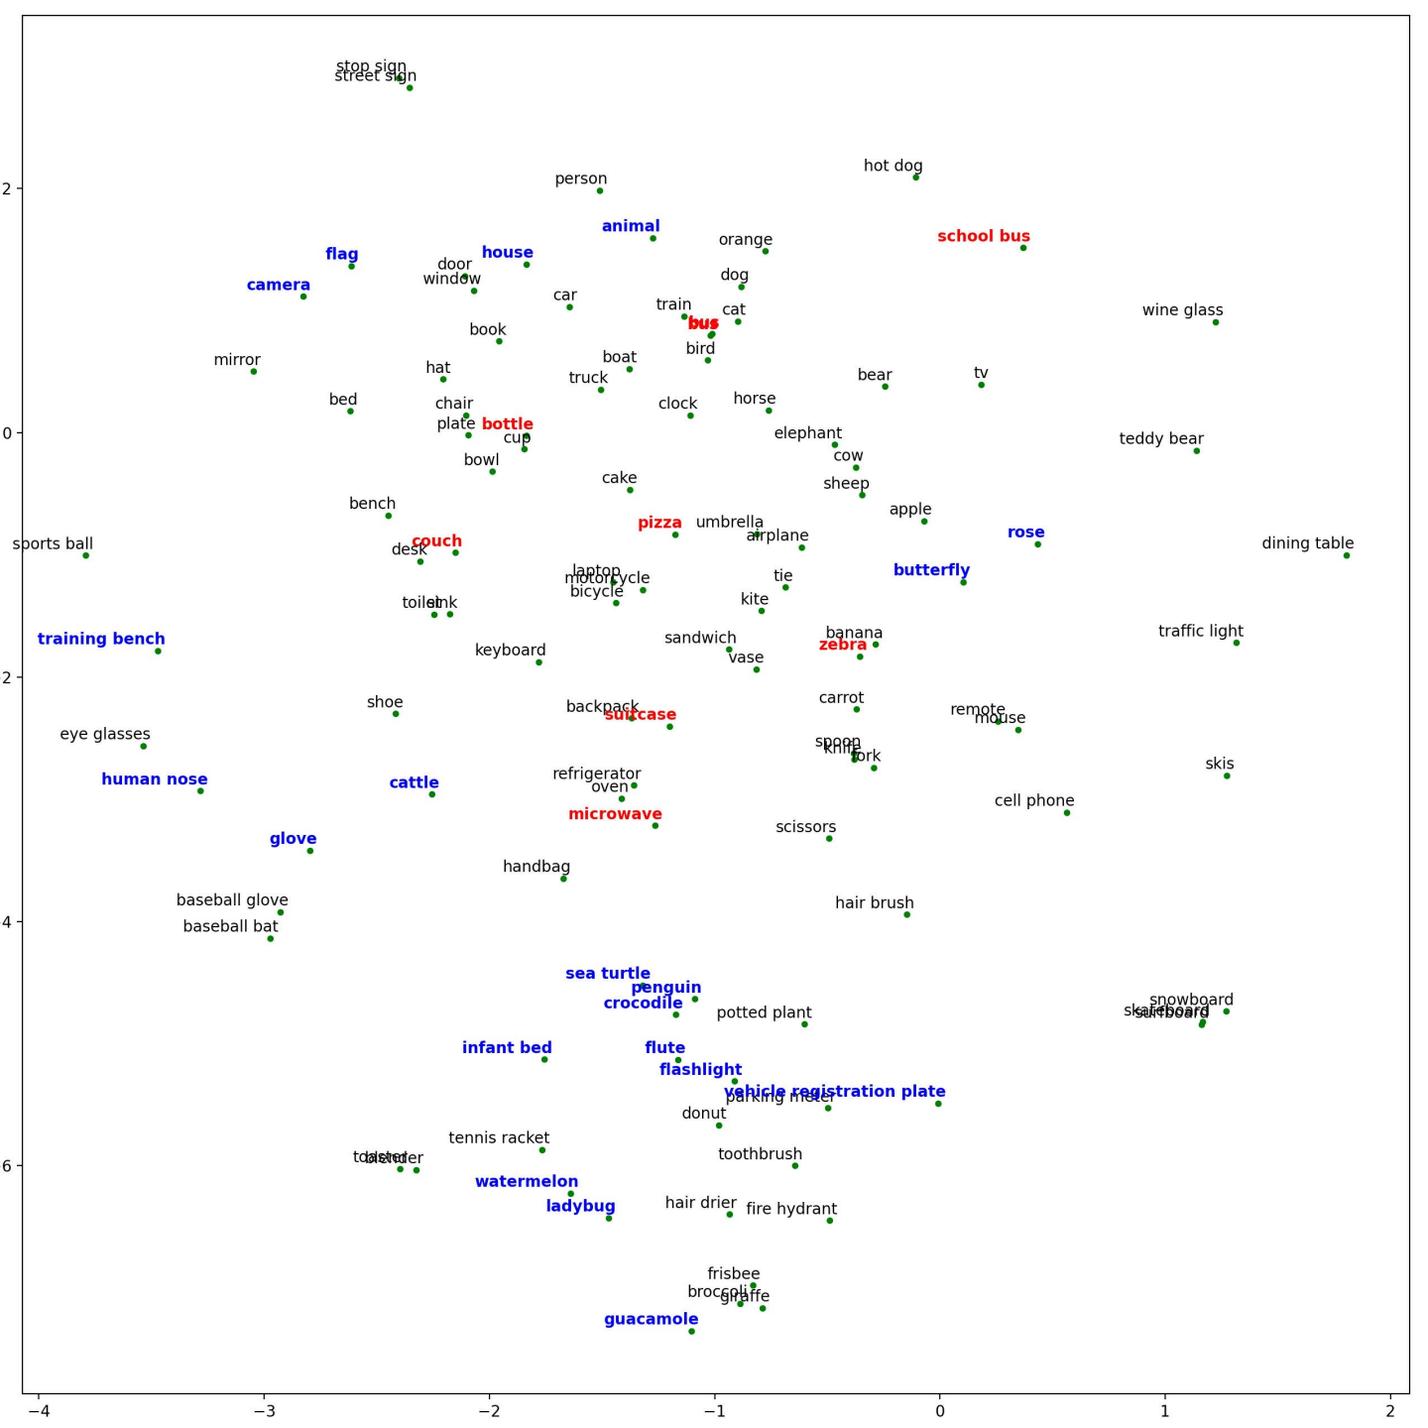



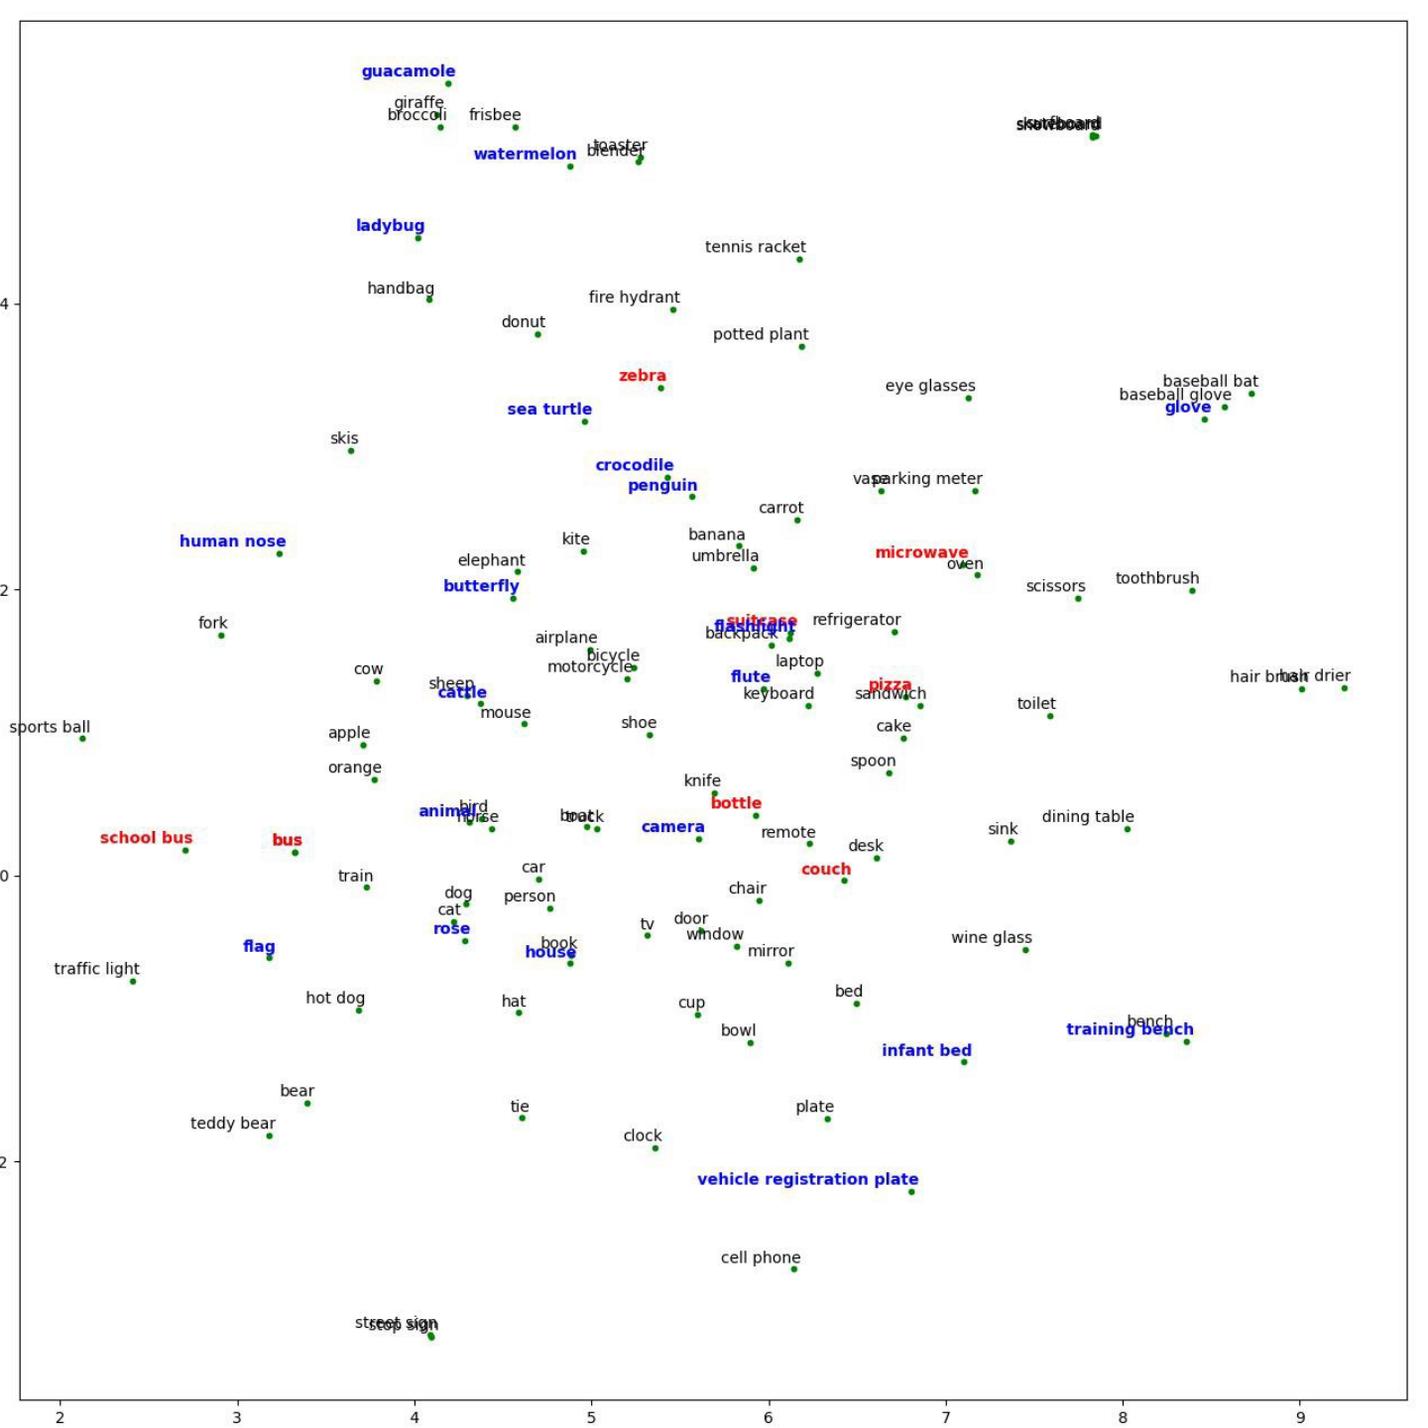

Supplement: Supplementary file 4 [file VIVO.pdf]
